# Supplementary material for: A Bayesian Network Model for Interesting Itemsets
Source: arXiv:1510.04130 ancillary file (2016-11-11)
Supplement: Supplementary file 1 [file supplementary.pdf]

# Supplementary Material for the Paper: A Bayesian Network Model for Interesting Itemsets

Jaroslav Fowkes*  Charles Sutton*

## 1 Introduction

This short report contains supplementary material for the accompanying paper: 'A Bayesian Network Model for Interesting Itemsets'. It consists of additional numerical results in the form of graphical depictions of the top itemsets as found by IIM, MTV, KRIMP and SLIM ranked according to the specified ranking for each method, i.e., interestingness, probability and usage, respectively.

## 2 Additional Numerical Experiments

***Plants Dataset*** As mentioned in the main paper, we ran IIM on the plants database [2]. In this database, each transaction is a species of plant and each item a U.S. or Canadian state where the plant is found. We would therefore expect correlated states to have similar flora and so occupy distinct geographical regions. This is exactly what we find in practice: among the top five itemsets, with an interestingness near 1, are {*Puerto Rico, Virgin Islands*}, {*California*} and {*Hawaii*} which all have a unique and very different flora compared to mainland North America. The other top interesting itemsets are similarly collections of states of various sizes which occupy geographically distinct and spatially coherent regions, the top four of which are depicted in Figure 1. Note how the top four itemsets contain both very small and very large collections of states.

Looking at the top itemsets as found by MTV, we find that they tend to be much smaller collections, averaging around 4 states, although the states do occupy spatially coherent regions as one would expect. The top four itemsets found by MTV are depicted in Figure 2. In particular, note that while MTV does return {*Puerto Rico*} as the top itemset, it does not associate it with the *Virgin Islands* (which are geographically adjacent) until the 20th ranked itemset. Similarly, the top itemsets found by KRIMP are also smaller collections of states and the top four are depicted in Figure 3. Like MTV, KRIMP also only finds the singleton {*Puerto Rico*} among the top ten itemsets, only associating it with the *Virgin Islands* in the 12th ranked itemset. Similarly, SLIM only does so in the 21st ranked itemset, the top four SLIM itemsets all being single states that occur frequently in the database as shown in Figure 4.

***Mammals Dataset*** Additionally, we ran IIM on the European mammals dataset [1]. Each transaction in the dataset is a roughly $50 \times 50$ km geographical grid cell and each item is a mammal that occurs in that grid cell. We would therefore expect the itemsets to be mammals that co-inhabit the same geographical regions and this is indeed what we find: the top itemsets found by IIM are groups of rarer mammals that co-inhabit small and very specific geographical regions, as we would expect from our interestingness ranking. For example, the top two non-singleton itemsets are a group of four mammals that coexist in Scotland and Ireland and a group of ten mammals that coexist on Sweden's border with Norway. In particular, the discovered itemsets correspond to very specific mammal correlations, e.g. {*Mountain Hare, Sika Deer, Grey Seal, Harbour Seal*} for the top itemset, even though this itemset is only present in 20 transactions. The top-four non-singleton IIM itemsets are shown in Figure 5 which depicts, for each itemset, the regions where the mammals in that itemset coexist.

By contrast, the top non-singleton itemsets as found by MTV are groups of more frequent mammals that co-inhabit relatively large areas of Europe, e.g. the top itemset returned by MTV is {*Eurasian Pygmy Shrew, Eurasian Water Shrew, Bank Vole, European Water Vole, Red Fox, Stoat, Least Weasel*} consisting of relatively common mammals that inhabit the majority of North-Western Europe. The top-four non-singleton MTV itemsets are shown in Figure 6 which depicts the regions where the mammals in each of the itemsets coexist. KRIMP is even less interesting in this respect, as the top mammal itemsets it returns are collections of some of the most common and well-known mammals in Europe, e.g. the 4th ranked KRIMP itemset is {*Wood Mouse, European Hedgehog, European Rabbit, House Mouse*}. The habitats of the mammals in each of the top-four non-singleton KRIMP itemsets are illustrated in Figure 7. SLIM behaves similarly to KRIMP in this respect, also returning collections of very common mammals e.g. {*European Otter, Red Deer*} as the 2nd ranked itemset. The top-four non-singleton SLIM itemsets are depicted in Figure 8.

*School of Informatics, University of Edinburgh, Edinburgh, EH8 9AB, UK, *email:* {jfowkes,csutton}@ed.ac.uk

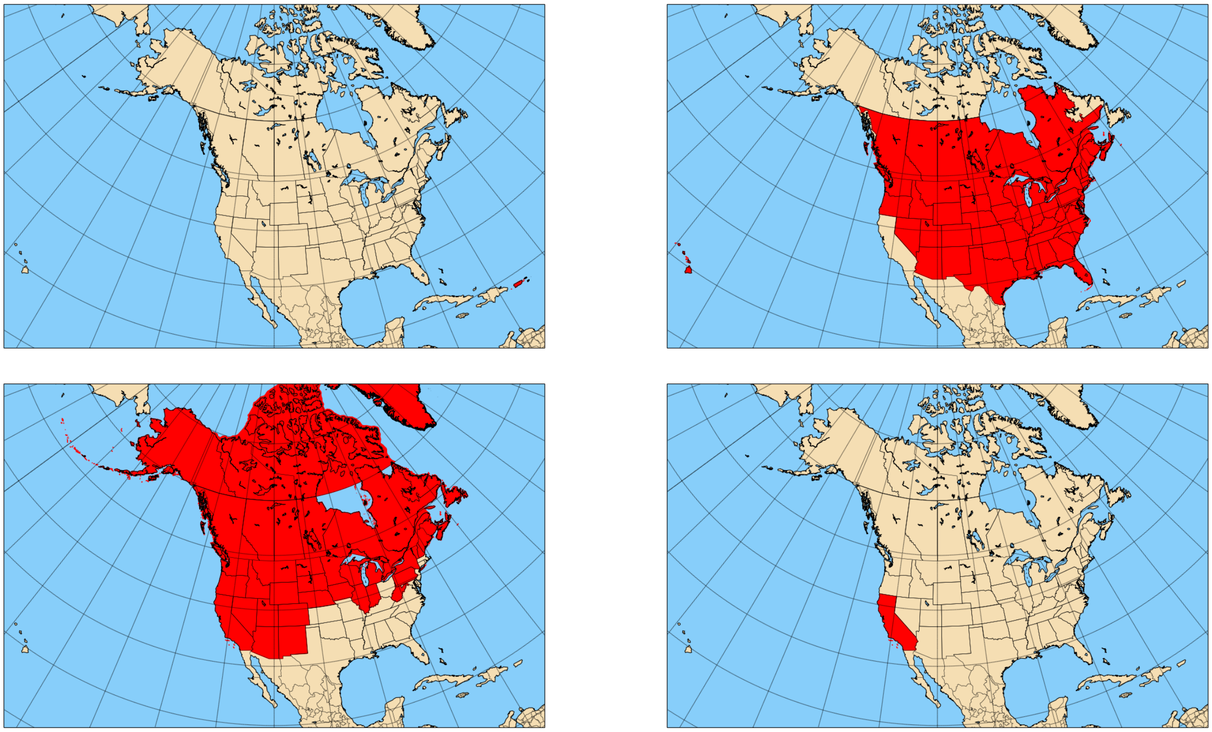

Figure 1: The top-four itemsets (groups of US/Canadian states) found by IIM for the plants dataset (top left is {*Puerto Rico, Virgin Islands*}). Note how they correspond to geographically distinct and spatially coherent regions, even though this information is not encoded in the model.

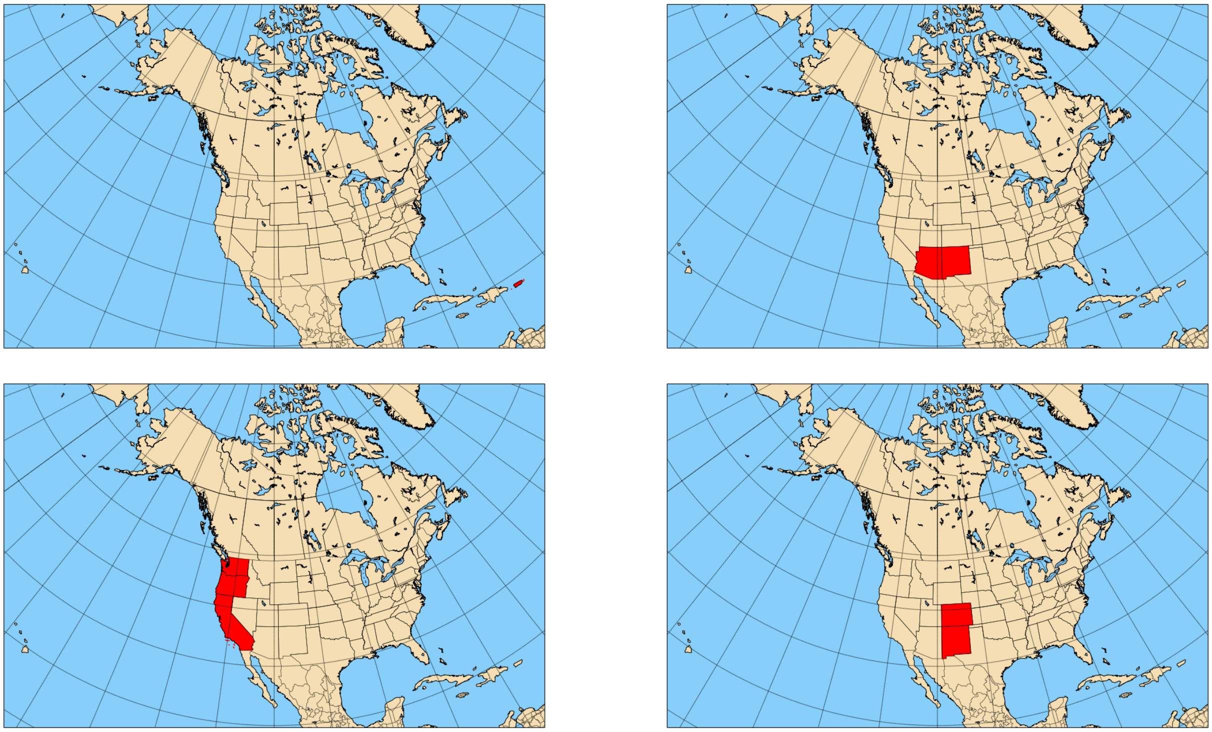

Figure 2: The top-four itemsets (groups of US/Canadian states) found by MTV for the plants dataset (top-left is {*Puerto Rico*}). Note that these are much smaller collections of states than those found by IIM and, unlike IIM, Virgin Islands is not associated with Puerto Rico.

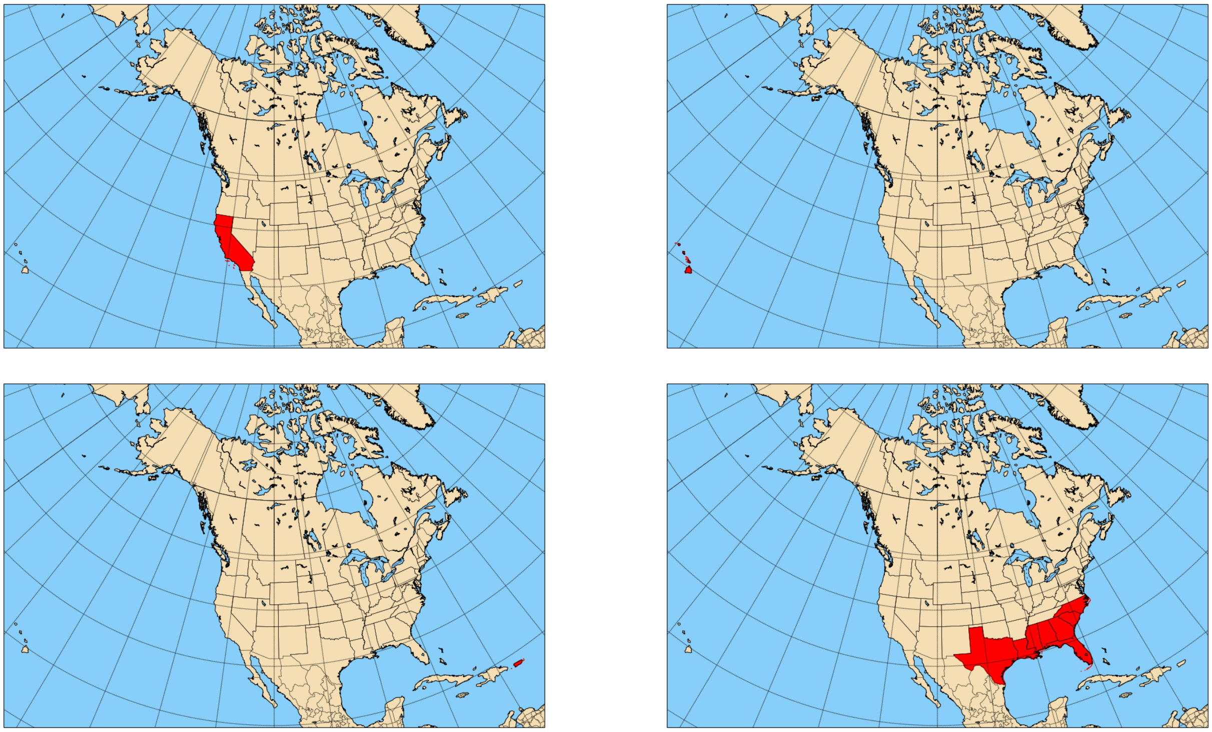

Figure 3: The top-four itemsets (groups of US/Canadian states) found by KRIMP for the plants dataset (top-right is {*Hawaii*}, bottom-left is {*Puerto Rico*}). Note that these are much smaller collections of states than those found by IIM and, unlike IIM, Virgin Islands is not associated with Puerto Rico.

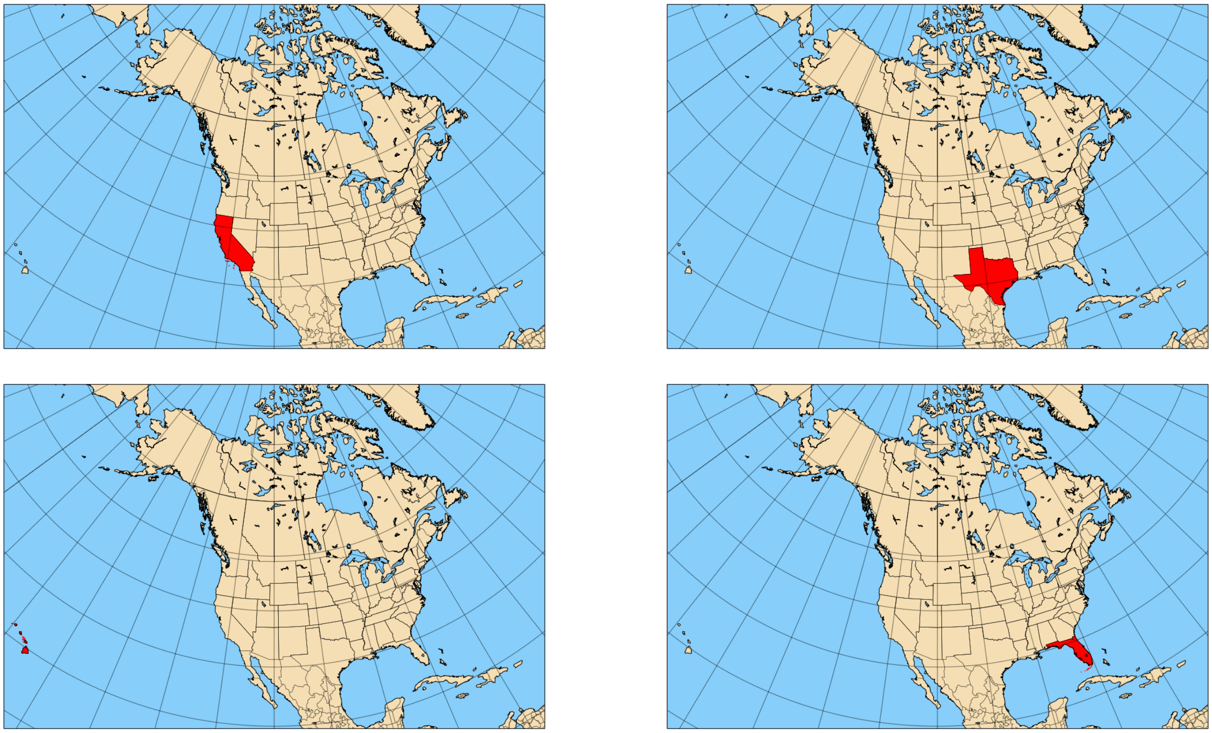

Figure 4: The top-four itemsets (groups of US/Canadian states) found by SLIM for the plants dataset (Top-left is {*California*}, top-right is {*Texas*}, bottom-left is {*Hawaii*}, and bottom-right is {*Florida*}). Note that these are all single states.

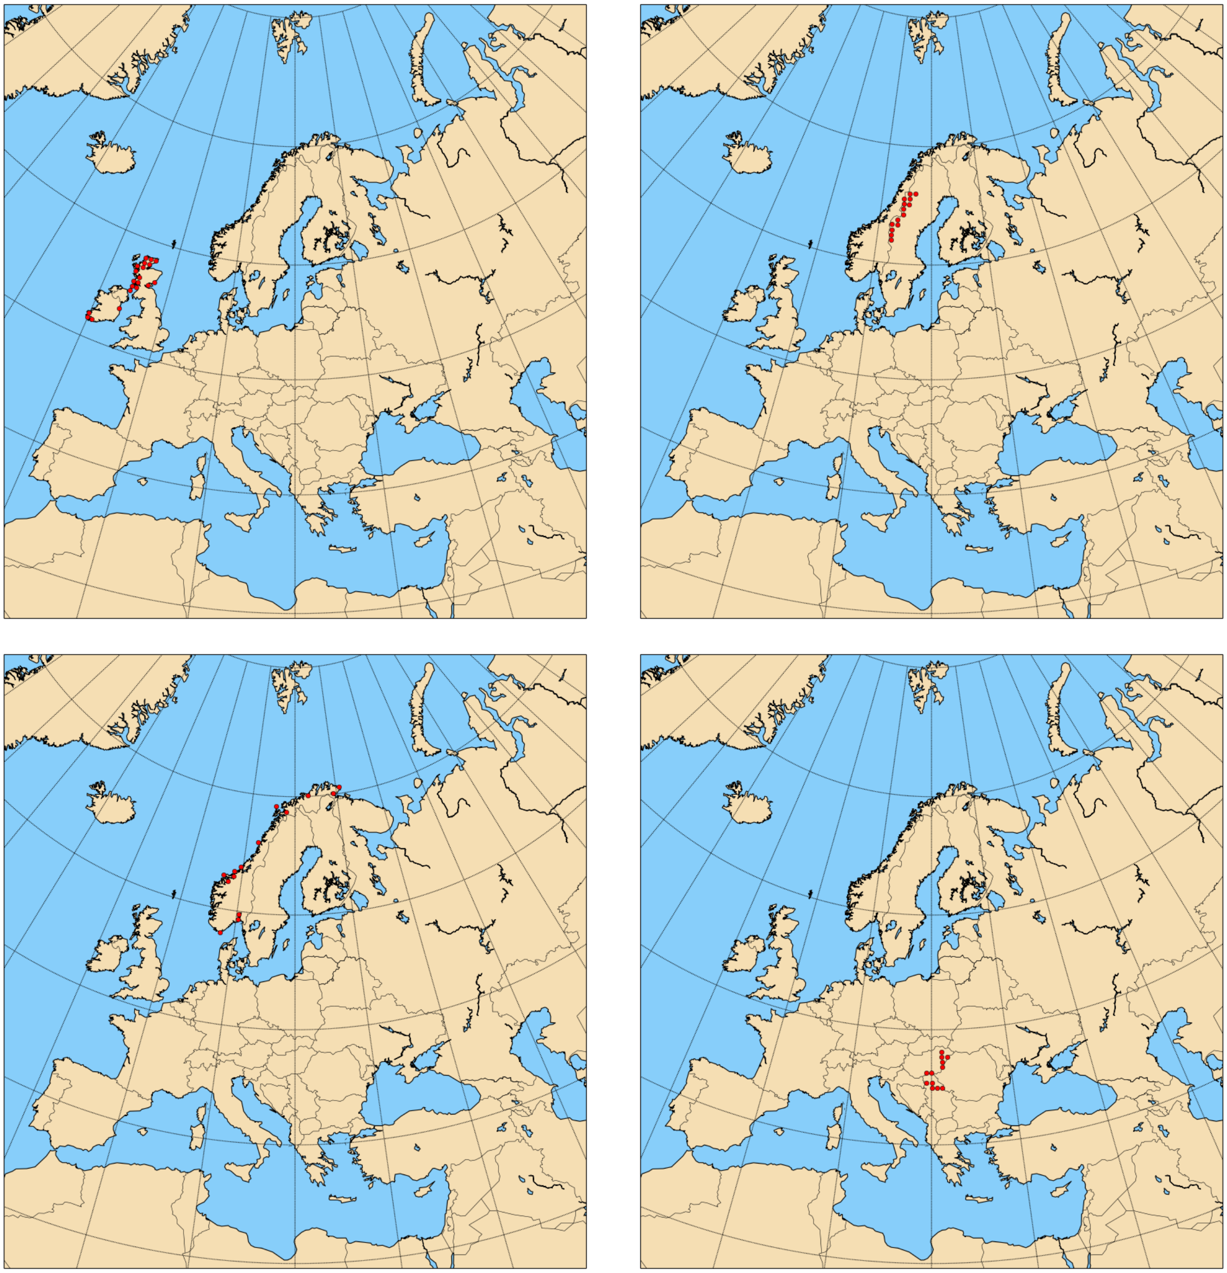

Figure 5: Geographical regions where the top-four non-singleton IIM itemsets of mammals coexist. Note how these correspond to groups of rarer mammals that co-inhabit small specific regions (as one would expect from our interestingness ranking), e.g. in the top-left: {*Mountain Hare, Sika Deer, Grey Seal, Harbor Seal*} and the bottom-left: {*Mountain Hare, Moose, Harbor Seal, Harp Seal*}. The other two itemsets are: Top-right: {*Northern Bat, Mountain Hare, Moose, Eurasian Lynx, Wood Lemming, Grey Red-backed Vole, Brown Bear, Norwegian Lemming, Arctic Fox, Wolverine*}, bottom-right: {*European Pine Vole, Wildcat, Bicolored Shrew, Southern White-breasted Hedgehog, Striped Field Mouse, European Ground Squirrel, European Hamster, Lesser Mole-rat, Steppe Mouse, Lesser White-toothed Shrew*}.

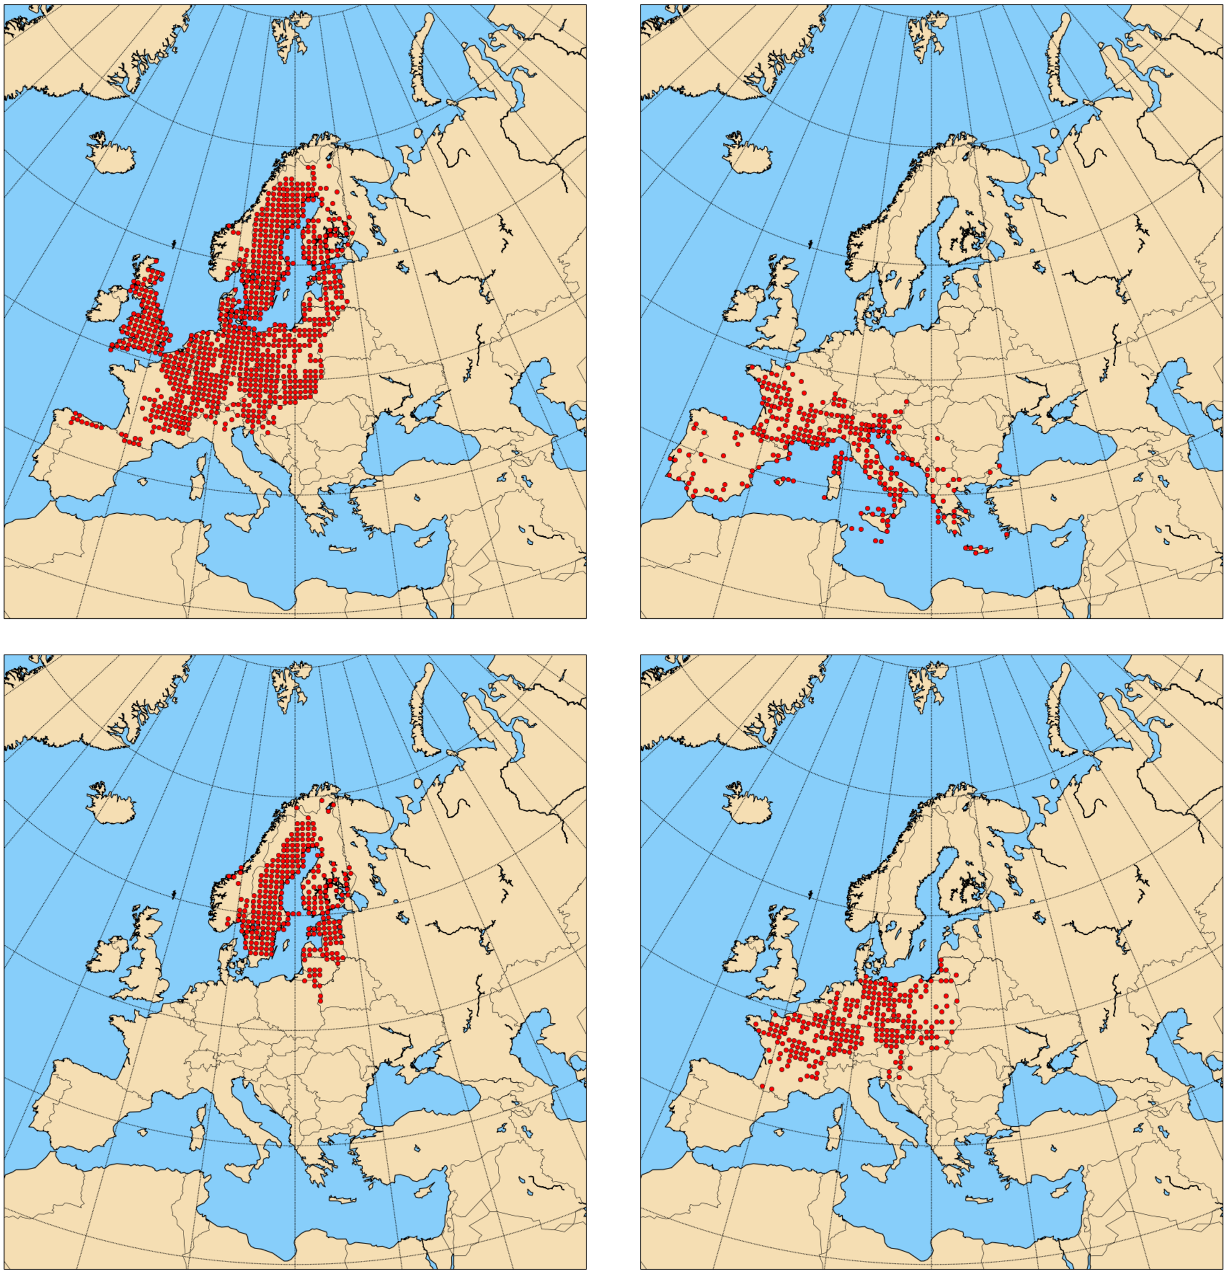

Figure 6: Geographical regions where the top-four non-singleton MTV itemsets of mammals coexist. In contrast to IIM, these correspond to groups of more frequent mammals that co-inhabit relatively large areas of Europe. The itemsets are as follows. Top-left: {*Eurasian Pygmy Shrew, Eurasian Water Shrew, Bank Vole, European Water Vole, Red Fox, Stoat, Least Weasel*}, top-right: {*Black Rat, Kuhl's pipistrelle*}, bottom-left: {*Red Squirrel, European Water Vole, Field Vole, Red Fox, Stoat, Common Shrew, European Pine Martin, Northern Bat, Mountain Hare, House Mouse, American Mink, Moose*}, bottom-right {*Eurasian Pygmy Shrew, Eurasian Water Shrew, European Mole, Daubenton's Bat, Serotine Bat, European Hare, Red Squirrel, Bank Vole, Muskrat, Field Vole, Common Vole, Eurasian Harvest Mouse, Wood Mouse, Brown Rat, Red Fox, Stoat, Least Weasel, European Polecat, Beech Marten, European Badger, Wild Boar, Roe Deer, Natterer's Bat, Brown Long-eared Bat, European Pine Marten*}.

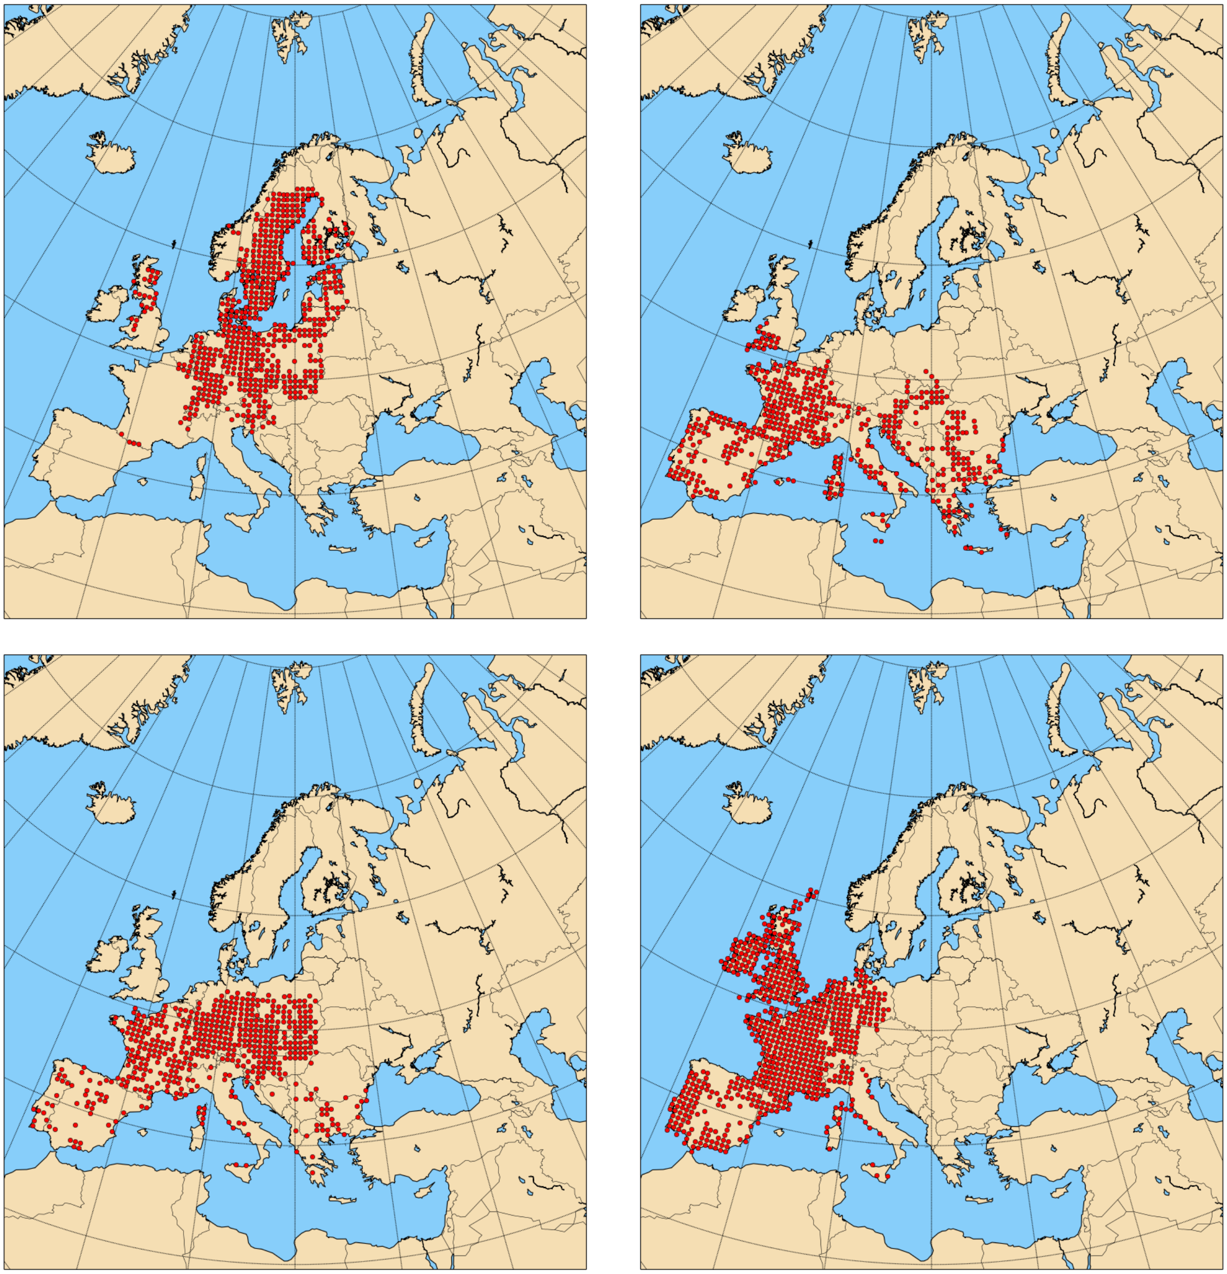

Figure 7: Geographical regions where the top-four non-singleton KRIMP itemsets of mammals coexist. In contrast to IIM, these correspond to groups of very common mammals that co-inhabit relatively large areas of Europe, e.g. in the bottom right: {*Wood Mouse, European Hedgehog, European Rabbit, House Mouse*}. The other itemsets are as follows. Top-left: {*Red Fox, Least Weasel, Brown Rat, European Badger, Red Squirrel, Roe Deer, Bank Vole, Eurasian Pygmy Shrew, Stoat, European Pine Marten, Field Vole, Common Shrew, Eurasian Water Shrew, European Water Vole*}, top-right: {*Lesser Horseshoe Bat, Greater Horseshoe Bat*}, bottom-left: {*Greater Mouse-eared Bat, Brown Long-eared Bat*}.

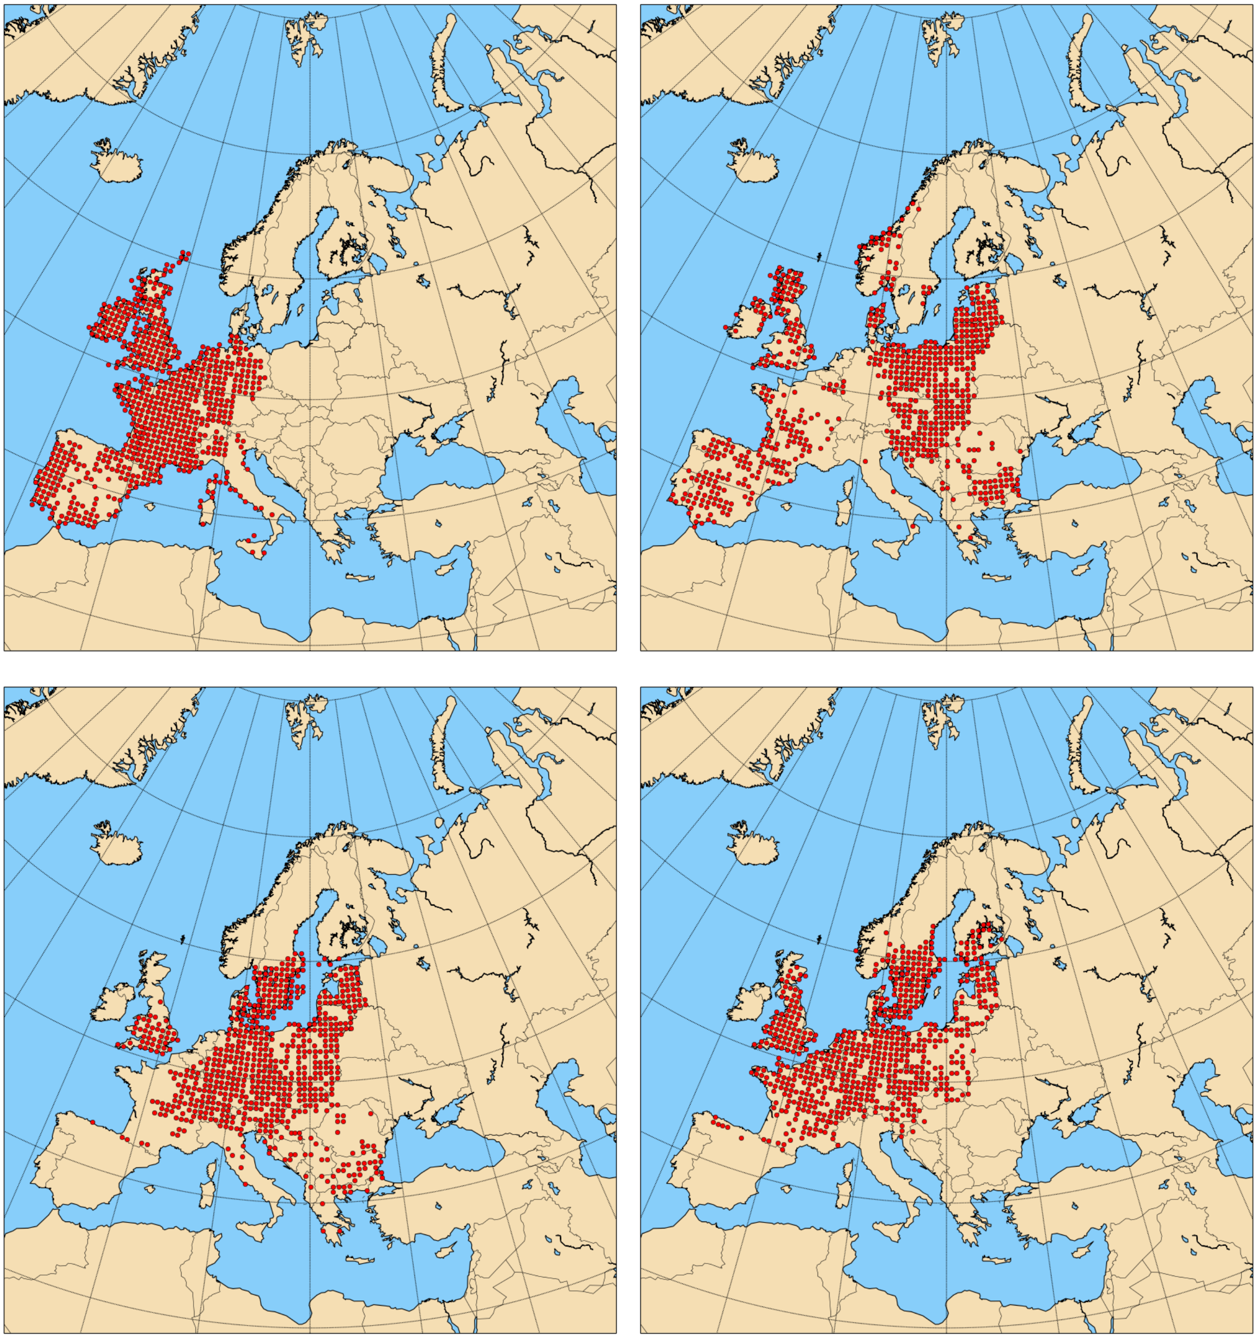

Figure 8: Geographical regions where the top-four non-singleton SLIM itemsets of mammals coexist. In contrast to IIM, these correspond to groups of very common mammals that co-inhabit relatively large areas of Europe, e.g. in the top left: {*European Hedgehog, European Rabbit, House Mouse*} and top-right: {*European Otter, Red Deer*}. The other itemsets are as follows. Bottom-left: {*Yellow-necked Mouse, Common Noctule*} and bottom-right: {*Bank Vole, Eurasian Pygmy Shrew, Stoat, Field Vole, Eurasian Water Shrew, Daubenton's Bat, Brown Long-eared Bat*}.

## References

[1] A. Mitchell-Jones, G. Amori, W. Bogdanowicz, B. Kryštufek, P. Reijnders, F. Spitzenberger, M. Stubbe, J. Thissen, V. Vohralík, and J. Zima. *The Atlas of European Mammals*. T & AD Poyser, 1999.

[2] USDA. The PLANTS Database, 2008.
